# Supplementary material for: Online Network Utility Maximization: Algorithm, Competitive Analysis, and Applications
Source: arXiv:2101.10898 source file (2021-01-26)
Supplement: Supplementary file 1 [file appendix.tex]

If the second assumption on the utility function is $g'_i(y)\in [m,M]$, we can also obtain an algorithm with the same competitive ratio by changing the :
\begin{algorithm}
\caption{Online Algorithm with Value Functions $\phi=\{\phi_\ell\}_{\ell\in \mathcal{L}}$ ($\text{OA}_\phi$)}
\begin{algorithmic}
\Initialize $\phi_\ell(\cdot),\forall \ell\in\mathcal{L}$, initial utilization $\omega^0_\ell = 0$;
\FOR{the $i$th arrival}
\STATE Observe the $i$th utility function $g_t(\cdot)$ and the $i$th set of link requested $\mathcal{L}_t$;
\STATE The network determine $y_t$ by solving the following utility maximization problem
$$ y_t= \text{argmax}_{0\le y\le b_t} \big\{ g_t(y) - \max_{\ell\in \mathcal{L}_t}\int_{\omega_\ell^{t-1}}^{\omega_\ell^{t-1}+y} \phi_\ell(s)ds \big\};$$
\STATE Update for links $\ell \in \mathcal{L}_t$: $\omega_\ell^t =  \omega_\ell^{t-1}+y_t;$
\ENDFOR
\end{algorithmic}
\end{algorithm}
